# Supplementary material for: Image Clustering via the Principle of Rate Reduction in the Age of Pretrained Models
Source: arXiv:2306.05272 source file (2024-04-26)
Supplement: Supplementary file 1 [file appendix_CIFAR10.tex]

\begin{figure*}[h]
  \centering
  \begin{subfigure}{0.32\textwidth}
    \includegraphics[width=\linewidth]{Fig/cluster-ours-CIFAR10/cluster_0.pdf}
    \caption{Learned cluster 1}
    % \caption{Input data $\calX$}
    % \label{fig:cifar10-1}
  \end{subfigure}
  \hfill
  \begin{subfigure}{0.32\textwidth}
    \includegraphics[width=\linewidth]{Fig/cluster-ours-CIFAR10/cluster_1.pdf}
    \caption{Learned cluster 2}
    % \caption{Input data $\calX$}
    % \label{fig:cifar10-2}
  \end{subfigure}
  \hfill
  \begin{subfigure}{0.32\textwidth}
    \includegraphics[width=\linewidth]{Fig/cluster-ours-CIFAR10/cluster_2.pdf}
    \caption{Learned cluster 3}
    % \caption{Input data $\calX$}
    % \label{fig:cifar10-3}
  \end{subfigure}
  \hfill
  \begin{subfigure}{0.32\textwidth}
    \includegraphics[width=\linewidth]{Fig/cluster-ours-CIFAR10/cluster_3.pdf}
    \caption{Learned cluster 4}
    % \caption{Input data $\calX$}
    % \label{fig:cifar10-4}
  \end{subfigure}
  \hfill
  \begin{subfigure}{0.32\textwidth}
    \includegraphics[width=\linewidth]{Fig/cluster-ours-CIFAR10/cluster_4.pdf}
    \caption{Learned cluster 5}
    % \caption{Input data $\calX$}
    % \label{fig:cifar10-5}
  \end{subfigure}
  \hfill
  \begin{subfigure}{0.32\textwidth}
    \includegraphics[width=\linewidth]{Fig/cluster-ours-CIFAR10/cluster_5.pdf}
    \caption{Learned cluster 6}
    % \caption{Input data $\calX$}
    % \label{fig:cifar10-6}
  \end{subfigure}
  \hfill
  \begin{subfigure}{0.32\textwidth}
    \includegraphics[width=\linewidth]{Fig/cluster-ours-CIFAR10/cluster_6.pdf}
    \caption{Learned cluster 7}
    % \caption{Input data $\calX$}
    % \label{fig:cifar10-7}
  \end{subfigure}
  \hfill
  \begin{subfigure}{0.32\textwidth}
    \includegraphics[width=\linewidth]{Fig/cluster-ours-CIFAR10/cluster_7.pdf}
    \caption{Learned cluster 8}
    % \caption{Input data $\calX$}
    % \label{fig:cifar10-8}
  \end{subfigure}
  \hfill
  \begin{subfigure}{0.32\textwidth}
    \includegraphics[width=\linewidth]{Fig/cluster-ours-CIFAR10/cluster_8.pdf}
    \caption{Learned cluster 9}
    % \caption{Input data $\calX$}
    % \label{fig:cifar10-9}
  \end{subfigure}
  \hfill
  \begin{subfigure}{0.32\textwidth}
    \includegraphics[width=\linewidth]{Fig/cluster-ours-CIFAR10/cluster_9.pdf}
    \caption{Learned cluster 10}
    % \caption{Input data $\calX$}
    % \label{fig:cifar10-9}
  \end{subfigure}
  \hfill
 
  \caption{Clusters learned by \ours{} on CIFAR10}
\end{figure*}

%-----------------------------------------------------------------------------------------------------------------------

\begin{figure*}[h]
  \centering
  \begin{subfigure}{0.32\textwidth}
    \includegraphics[width=\linewidth]{Fig/cluster-clip-CIFAR10/cluster_0.pdf}
    \caption{Learned cluster 1}
    % \caption{Input data $\calX$}
    % \label{fig:cifar10-1}
  \end{subfigure}
  \hfill
  \begin{subfigure}{0.32\textwidth}
    \includegraphics[width=\linewidth]{Fig/cluster-clip-CIFAR10/cluster_1.pdf}
    \caption{Learned cluster 2}
    % \caption{Input data $\calX$}
    % \label{fig:cifar10-2}
  \end{subfigure}
  \hfill
  \begin{subfigure}{0.32\textwidth}
    \includegraphics[width=\linewidth]{Fig/cluster-clip-CIFAR10/cluster_2.pdf}
    \caption{Learned cluster 3}
    % \caption{Input data $\calX$}
    % \label{fig:cifar10-3}
  \end{subfigure}
  \hfill
  \begin{subfigure}{0.32\textwidth}
    \includegraphics[width=\linewidth]{Fig/cluster-clip-CIFAR10/cluster_3.pdf}
    \caption{Learned cluster 4}
    % \caption{Input data $\calX$}
    % \label{fig:cifar10-4}
  \end{subfigure}
  \hfill
  \begin{subfigure}{0.32\textwidth}
    \includegraphics[width=\linewidth]{Fig/cluster-clip-CIFAR10/cluster_4.pdf}
    \caption{Learned cluster 5}
    % \caption{Input data $\calX$}
    % \label{fig:cifar10-5}
  \end{subfigure}
  \hfill
  \begin{subfigure}{0.32\textwidth}
    \includegraphics[width=\linewidth]{Fig/cluster-clip-CIFAR10/cluster_5.pdf}
    \caption{Learned cluster 6}
    % \caption{Input data $\calX$}
    % \label{fig:cifar10-6}
  \end{subfigure}
  \hfill
  \begin{subfigure}{0.32\textwidth}
    \includegraphics[width=\linewidth]{Fig/cluster-clip-CIFAR10/cluster_6.pdf}
    \caption{Learned cluster 7}
    % \caption{Input data $\calX$}
    % \label{fig:cifar10-7}
  \end{subfigure}
  \hfill
  \begin{subfigure}{0.32\textwidth}
    \includegraphics[width=\linewidth]{Fig/cluster-clip-CIFAR10/cluster_7.pdf}
    \caption{Learned cluster 8}
    % \caption{Input data $\calX$}
    % \label{fig:cifar10-8}
  \end{subfigure}
  \hfill
  \begin{subfigure}{0.32\textwidth}
    \includegraphics[width=\linewidth]{Fig/cluster-clip-CIFAR10/cluster_8.pdf}
    \caption{Learned cluster 9}
    % \caption{Input data $\calX$}
    % \label{fig:cifar10-9}
  \end{subfigure}
  \hfill
  \begin{subfigure}{0.32\textwidth}
    \includegraphics[width=\linewidth]{Fig/cluster-clip-CIFAR10/cluster_9.pdf}
    \caption{Learned cluster 10}
    % \caption{Input data $\calX$}
    % \label{fig:cifar10-9}
  \end{subfigure}
  \hfill
 
  \caption{Clusters with KMeans and Original CLIP features on CIFAR10}
\end{figure*}
